# Supplementary material for: MGStream: Motion-aware 3D Gaussian for Streamable Dynamic Scene Reconstruction
Source: arXiv:2505.13839 source file (2025-05-20)
Supplement: Supplementary file 1 [file supple.tex]

\clearpage
\setcounter{page}{1}

\maketitlesupplementary

\section{Summary}\label{summary}
In this appendix, we present further materials to support and extend our method and experiments presented in the main body of this paper. 
This supplementary material is organized as follows:
\begin{itemize}
    \item \cref{more_details} presents the implementation details and interpretation of the proposed method.
    
    \item \cref{more_results} provides i) the per-scene breakdown of the quantitative evaluation from \cref{table:comparison_table_online}, 
    ii) the qualitative results of \cref{table:Ablation_architecture,table:Ablation_NOL},
    iii) the visualization of dynamic regions used for PSNR calculations on \cref{table:comparison_table_online}, 
    and iv) the number of motion-related 3DGs in different N3DV scenes.

    \item \cref{more_ablation_study} presents more ablation studies on 
    i) the individual components,
    ii) the optical flow mask, 
    iii) the hyper-parameter ($\epsilon$) in the clustering algorithm,
    iv) the GIM,
    v) the motion-related 3DGs.

    \item Furthermore, a supplementary video is attached as qualitative comparisons.
\end{itemize}

% \cref{more_results} provides comprehensive experimental results, followed by additional ablation studies in \cref{more_ablation_study}.
% Furthermore, We include supplementary videos demonstrating qualitative comparisons.

\section{More Details}
\label{more_details}
\textit{Overview}.
In this section, we elaborate on several key technical components, encompassing both conceptual refinements (\textit{Motion-related 3DGs} and \textit{Mapping Function}) and qualitative demonstrations (\textit{Cluster-based Convex Hull Algorithm}, and \textit{Attention Map}).

\textit{Motion-related 3DGs}.
The motion-related 3DGs ($G_m$) are used for modeling the dynamic in the proposed method. It is comprised of the motion-related 3DGs obtained via back-projection ($G_o$) and the motion-related 3DGs corresponding to the inside part of the moving object $G_i$.  $G_{new}$ represents the motion-related 3DGs responsible for the emerging objects.
% MGStream utilizes the motion-related 3DGs ($G_m$) for modeling the dynamic, and the vanilla 3DGs for the static. The motion-related 3DGs ($G_m$) include two subsets: motion-related 3DGs obtained with back-projection $G_o$ and motion-related 3DGs corresponding to inside parts of the moving object $G_i$. In addition, there is a subset of $G_m$ that responsible for the emerging objects $G_{new}$ based on our proposed attention map $M_a$.
% The following sections detail some key technical components: \textit{GIM Map}, \textit{Mapping Function}, \textit{Cluster-based Convex Hull Algorithm}, and the \textit{Attention Map}.

\textit{Mapping Function}.
Two mapping functions, $\mathcal{F}_d$ and $\mathcal{F}_c$ are used to estimate the deformation and color parameters, respectively. $\mathcal{F}_d$ outputs 7-dimensional deformation offsets ($\Delta u_t$, $\Delta q_t$), and $\mathcal{F}_c$ predicts 12-dimensional optimization offsets ($\Delta sh_t$).
Specifically, the mapping functions $\mathcal{F}_d$ and $\mathcal{F}_c$ are implemented via two independent hash grids coupled with different lightweight MLPs.  Each hash grid incorporates 16 levels, ranging from the coarsest resolution of 16 to the finest resolution of $2^9$, with a table size of $2^{15}$. At each level, a 4-dimensional feature vector is interpolated, resulting in a concatenated 64-dimensional feature vector. For the deformation phase, the lightweight MLPs comprise two hidden layers and one output layer, utilizing the ReLU activation function. The two hidden layers both have 64 neurons and the output layer has 7 neurons, respectively. It takes the 64-dimensional hash features as input and outputs 7-dimensional rotation and translation offsets ($\Delta u_t$, $\Delta q_t$). For the optimization phase, the lightweight MLP has a similar structure, and the only difference is that it has 12 neurons for the last MLP layer to output 12-dimensional spherical harmonic coefficients offsets ($\Delta sh_t$).

\begin{figure}[t!]   % \begin{figure}[ht!]
	\centering
	\begin{subfigure}{\linewidth}
            % \rotatebox[origin=c]{90}{\footnotesize{Results}\hspace{-1.3cm}}
            \begin{minipage}[t]{0.32\linewidth}
                \centering
                \includegraphics[width=1\linewidth]{figure_supple/sup2_group/fig1.png}
                % \caption{Full}
                \caption{Images}
            \end{minipage}
            \begin{minipage}[t]{0.32\linewidth}
                \centering
                \includegraphics[width=1\linewidth]{figure_supple/sup2_group/fig2.png}
                % \caption{GIM}
                \caption{$G_m$ w/o CA.}
            \end{minipage}
            \begin{minipage}[t]{0.32\linewidth}
                \centering
                \includegraphics[width=1\linewidth]{figure_supple/sup2_group/fig3.png}
                % \caption{Rendered image}
                \caption{$G_m$ with CA}
            \end{minipage}
        \end{subfigure}

       \caption{Comparison of the motion-related 3DGs $G_m$ obtained using the methods with/without our clustering algorithm. CA means Clustering Algorithm. It is clearly seen that removing the CA would misclassify some vanilla 3DGs as motion-related 3DGs, \eg the glass bottles between the man and the dog.}
       % \vspace{1em}
       \label{fig:Clustering}   
\end{figure}

\begin{figure}[t!]   % \begin{figure}[ht!]
	\centering
	\begin{subfigure}{\linewidth}
            % \rotatebox[origin=c]{90}{\footnotesize{Results}\hspace{-1.3cm}}
            \begin{minipage}[t]{0.32\linewidth}
                \centering
                \includegraphics[width=1\linewidth]{figure_supple/sup3_attention/fig1.png}
                % \caption{Full}
                \caption{GT}
            \end{minipage}
            \begin{minipage}[t]{0.32\linewidth}
                \centering
                \includegraphics[width=1\linewidth]{figure_supple/sup3_attention/fig2.png}
                % \caption{GIM}
                \caption{deformation}
            \end{minipage}
            \begin{minipage}[t]{0.32\linewidth}
                \centering
                \includegraphics[width=1\linewidth]{figure_supple/sup3_attention/fig3.png}
                % \caption{Rendered image}
                \caption{attention map}
            \end{minipage}
        \end{subfigure}
       \caption{Illustration of the attention map. (a), (b) are the ground truth image and the rendered image after deformation, respectively. The red-highlighted areas in (c) represent the attention map, indicating regions of the emerging objects.}
       \vspace{-0.5em}
       \label{fig:Attention}   
\end{figure}

\textit{Clustering-based Convex Hull Algorithm}. 
The proposed clustering-based convex hull algorithm first conducts the clustering operation, and then performs Delaunay Triangulation \cite{DBSCAN} on the motion-related 3DGs via back-projection $G_o$, establishing a convex hull structure that minimizes the occurrence of sliver triangles. 
As seen in \cref{fig:Clustering}, the clustering operation is essential for identifying the motion-related 3DGs. The 3DGs between two dynamic objects, responsible for the static,  would be classified as motion-related 3DGs when removing the clustering operation.

\textit{Attention Map}. 
To locate the motion-related 3DGs responsible for emerging objects ($G_{new}$), we compute the attention map via the maximum pixel-wise rendering errors using the deformed 3DGs. As demonstrated in \cref{fig:Attention}, our attention map finds $G_{new}$ and constrains them with pixel loss for learning the correct spherical harmonic coefficient, thus contributing to the modeling of the emerging objects.

\begin{figure*}[ht!]
	\centering

	\begin{subfigure}{\linewidth}
            \begin{minipage}[t]{0.193\linewidth}
                \centering
                \includegraphics[width=1\linewidth]{figure_supple/sup4_dynamic/fig1_coffee_martini.png}
                \caption{coffee\_martini}
            \end{minipage}
            \begin{minipage}[t]{0.193\linewidth}
                \centering
                \includegraphics[width=1\linewidth]{figure_supple/sup4_dynamic/fig2_cook_spinach.png}
                \caption{cook\_spinach}
            \end{minipage}
            \begin{minipage}[t]{0.193\linewidth}
                \centering
                \includegraphics[width=1\linewidth]{figure_supple/sup4_dynamic/fig3_cut_roasted_beef.png}
                \caption{cut\_roasted\_beef}
            \end{minipage}
            \begin{minipage}[t]{0.193\linewidth}
                \centering
                \includegraphics[width=1\linewidth]{figure_supple/sup4_dynamic/fig5_flame_salmon_1.png}
                \caption{flame\_salmon}
            \end{minipage}
            \begin{minipage}[t]{0.193\linewidth}
                \centering
                \includegraphics[width=1\linewidth]{figure_supple/sup4_dynamic/fig6_flame_steak.png}
                \caption{flame\_steak}
            \end{minipage}
        \end{subfigure}

	\begin{subfigure}{\linewidth}
            \begin{minipage}[t]{0.193\linewidth}
                \centering
                \includegraphics[width=1\linewidth]{figure_supple/sup4_dynamic/fig7_sear_steak.png}
                \caption{sear\_steak}
            \end{minipage}
            \begin{minipage}[t]{0.193\linewidth}
                \centering
                \includegraphics[width=1\linewidth]{figure_supple/sup4_dynamic/fig4_discussion.png}
                \caption{discussion}
            \end{minipage}
            \begin{minipage}[t]{0.193\linewidth}
                \centering
                \includegraphics[width=1\linewidth]{figure_supple/sup4_dynamic/fig8_stepin.png}
                \caption{stepin}
            \end{minipage}
            \begin{minipage}[t]{0.193\linewidth}
                \centering
                \includegraphics[width=1\linewidth]{figure_supple/sup4_dynamic/fig9_trimming.png}
                \caption{trimming}
            \end{minipage}
            \begin{minipage}[t]{0.193\linewidth}
                \centering
                \includegraphics[width=1\linewidth]{figure_supple/sup4_dynamic/fig10_vrheadset.png}
                \caption{vrheadset}
            \end{minipage}
        \end{subfigure}
        % \vspace{-0.3cm}
	\caption{Illustration of the dynamic regions.
    }
	\label{fig:dynamic_region}
\end{figure*}

\begin{table*}[ht!]
\caption{Quantitative comparison with online methods across all
scenes on the N3DV and MeetRoom datasets. 
PSNR($\cdot$ / $\cdot$) means the PSNR calculated using the entire image and the dynamic region, respectively. 
Storage($\cdot$ / $\cdot$) means the storage calculation includes and excludes the initial frame, respectively.
\colorbox{Magenta!30}{Pink} and \colorbox{Melon!40}{Brown} indicate the best and the second, respectively. * means re-implementing the experiments with identical initiation 3DGs as ours. $^{\dag}$ means the results obtained in our experiments with the official codes.} 
\label{table:supple_comparison_table_online}
\centering 
\begin{tabular}{c | c c c c c c}
\Xhline{3\arrayrulewidth}

\multirow{2}{*}{Method} & \multicolumn{3}{c}{Coffee Martini} & \multicolumn{3}{c}{Cook Spinach} \\
& PSNR ($\cdot$ / $\cdot$) $\uparrow$ & Storage ($\cdot$ / $\cdot$) (MB)$\downarrow$ & $E_{warp}\downarrow $ & PSNR ($\cdot$ / $\cdot$) $\uparrow$ & Storage ($\cdot$ / $\cdot$) (MB)$\downarrow$ & $E_{warp}\downarrow$ \\

StreamRF$^{\dag}$ & \cellcolor{Melon!40}{28.36 / 27.36} & 24.25 / 29.75 & \cellcolor{Melon!40}{0.0114} & 31.55 / 30.74 & 18.56 / 24.68 & \cellcolor{Melon!40}{0.0105} \\
Dynamic3DGS$^{\dag}$ & 24.70 / 24.42 & 14.14 / 14.28 & 0.0388 & 31.16 / 30.92 & 9.35 / 9.43 & 0.0248 \\
3DGStream$^*$ & 28.30 / 26.13 & \cellcolor{Melon!40}{7.60 / 7.77} & 0.0119 & \cellcolor{Melon!40}{33.09 / 30.56} & \cellcolor{Melon!40}{7.60 / 7.69} & 0.0129 \\
Ours & \cellcolor{Magenta!30}{28.42 / 26.41} & \cellcolor{Magenta!30}{2.52 / 2.70} & \cellcolor{Magenta!30}{0.0088} &  \cellcolor{Magenta!30}{33.34 / 31.06} & \cellcolor{Magenta!30}{1.87 / 1.98} & \cellcolor{Magenta!30}{0.0103} \\
    
% \Xhline{3\arrayrulewidth}
\hline
\multirow{2}{*}{Method} & \multicolumn{3}{c}{Cut Roasted Beef} & \multicolumn{3}{c}{Flame Salmon} \\
& PSNR ($\cdot$ / $\cdot$) $\uparrow$ & Storage ($\cdot$ / $\cdot$) (MB)$\downarrow$ & $E_{warp}\downarrow $ & PSNR ($\cdot$ / $\cdot$) $\uparrow$ & Storage ($\cdot$ / $\cdot$) (MB)$\downarrow$ & $E_{warp}\downarrow$ \\
StreamRF$^{\dag}$ & 31.28 / 30.92 & 18.96 / 25.05 & \cellcolor{Magenta!30}{0.0121} & 28.36 / 26.45 & 22.13 / 25.55 & \cellcolor{Melon!40}{0.0097} \\
Dynamic3DGS$^{\dag}$ & 30.84 / 32.02 & 9.01 / 9.08 & 0.0257 & 25.38 / 24.01 & 17.22 / 17.36 & 0.0339 \\
3DGStream$^*$ & \cellcolor{Melon!40}{33.63 / 32.53} & \cellcolor{Melon!40}{7.60 / 7.67} & 0.0144 & \cellcolor{Melon!40}{28.41 / 25.93} & \cellcolor{Melon!40}{7.60 / 7.77} & 0.0115 \\
Ours & \cellcolor{Magenta!30}{33.69 / 32.80} & \cellcolor{Magenta!30}{1.83 / 1.92} & \cellcolor{Magenta!30}{0.0121} & \cellcolor{Magenta!30}{28.70 / 26.04} & \cellcolor{Magenta!30}{2.72 / 2.91} & \cellcolor{Magenta!30}{0.0087} \\

% \Xhline{3\arrayrulewidth}
\hline
\multirow{2}{*}{Method} & \multicolumn{3}{c}{Flame Steak} & \multicolumn{3}{c}{Sear Steak} \\
& PSNR ($\cdot$ / $\cdot$) $\uparrow$ & Storage ($\cdot$ / $\cdot$) (MB)$\downarrow$ & $E_{warp}\downarrow $ & PSNR ($\cdot$ / $\cdot$) $\uparrow$ & Storage ($\cdot$ / $\cdot$) (MB)$\downarrow$ & $E_{warp}\downarrow$ \\
StreamRF$^{\dag}$ & 32.14 / 31.89 & 17.87 / 23.72 & \cellcolor{Magenta!30}{0.0092} & 32.27 / 33.30 & 17.32 / 23.10 & \cellcolor{Magenta!30}{0.0090} \\
Dynamic3DGS$^{\dag}$ & 32.94 / 32.12 & 8.32 / 8.39 & 0.0205 & \cellcolor{Melon!40}{33.50 / 34.72} & 8.66 / 8.74 & 0.0229 \\
3DGStream$^*$ & \cellcolor{Melon!40}{34.20 / 33.19} & \cellcolor{Melon!40}{7.60 / 7.67} & 0.0123 & 33.39 / 34.00 & 7.60 / 7.68 & 0.0117 \\
Ours & \cellcolor{Magenta!30}{34.31 / 33.45} & \cellcolor{Magenta!30}{1.80 / 1.89} & \cellcolor{Melon!40}{0.0104} & \cellcolor{Magenta!30}{33.62 / 34.92} & \cellcolor{Magenta!30}{1.76 / 1.86} & \cellcolor{Melon!40}{0.0097} \\

% \Xhline{3\arrayrulewidth}
\hline
\multirow{2}{*}{Method} & \multicolumn{3}{c}{Discussion} & \multicolumn{3}{c}{Stepin} \\
& PSNR ($\cdot$ / $\cdot$) $\uparrow$ & Storage ($\cdot$ / $\cdot$) (MB)$\downarrow$ & $E_{warp}\downarrow $ & PSNR ($\cdot$ / $\cdot$) $\uparrow$ & Storage ($\cdot$ / $\cdot$) (MB)$\downarrow$ & $E_{warp}\downarrow$ \\
StreamRF$^{\dag}$ & 29.33 / 27.04 & 4.62 / 8.43 & \cellcolor{Melon!40}{0.0087} & 27.17 / 26.94 & 5.62 / 9.89 & 0.0159 \\
Dynamic3DGS$^{\dag}$ & 29.07 / 27.05 & 4.62 / 4.65 & 0.0229 & 27.16 / 28.99 & \cellcolor{Melon!40}{3.60 / 3.63} & 0.0297 \\
3DGStream$^*$ & \cellcolor{Melon!40}{30.81 / 28.99} & \cellcolor{Melon!40}{4.00 / 4.03} & 0.0104 & \cellcolor{Melon!40}{28.34 / 27.76} & {4.00 / 4.03} & \cellcolor{Magenta!30}{0.0128} \\
Ours & \cellcolor{Magenta!30}{31.82 / 29.45} & \cellcolor{Magenta!30}{1.07 / 1.11} & \cellcolor{Magenta!30}{0.0075} & \cellcolor{Magenta!30}{29.31 / 28.96} & \cellcolor{Magenta!30}{0.72 / 0.76} & \cellcolor{Melon!40}{0.0153} \\
    
% \Xhline{3\arrayrulewidth}
\hline
\multirow{2}{*}{Method} & \multicolumn{3}{c}{Trimming} & \multicolumn{3}{c}{Vrheadset} \\
& PSNR ($\cdot$ / $\cdot$) $\uparrow$ & Storage ($\cdot$ / $\cdot$) (MB)$\downarrow$ & $E_{warp}\downarrow $ & PSNR ($\cdot$ / $\cdot$) $\uparrow$ & Storage ($\cdot$ / $\cdot$) (MB)$\downarrow$ & $E_{warp}\downarrow$ \\
StreamRF$^{\dag}$ & 29.22 / 28.32 & 4.19 / 8.48 & \cellcolor{Magenta!30}{0.0085} & 28.84 / 27.81 & 4.29 / 8.56 & \cellcolor{Melon!40}{0.0064} \\ 
Dynamic3DGS$^{\dag}$ & 27.49 / 27.49 & \cellcolor{Melon!40}{3.25 / 3.28} & 0.0249 & 28.04 / 26.77 & 3.94 / 3.97 & 0.0225 \\
3DGStream$^*$ & \cellcolor{Melon!40}{31.46 / 31.24} & 4.00 / 4.02 & 0.0105 & \cellcolor{Melon!40}{30.31 / 29.51} & \cellcolor{Melon!40}{4.00 / 4.03} & 0.0102 \\
Ours & \cellcolor{Magenta!30}{31.73 / 31.35} & \cellcolor{Magenta!30}{0.62 / 0.66} & \cellcolor{Melon!30}{0.0087} & \cellcolor{Magenta!30}{31.85 / 30.61} & \cellcolor{Magenta!30}{0.58 / 0.62} & \cellcolor{Magenta!30}{0.0057} \\

\Xhline{3\arrayrulewidth}
\end{tabular}
\end{table*}

\textit{Delaunay Triangulation (DT)}.
DT constructs a triangulation for a given 3D points set ($P$). The input is the $P$ set, and the output is a mesh connecting these points. DT is based on the empty circle criterion: for any constructed triangle, its circumcircle must contain no other points from the $P$ set, which ensures the triangles are as "well-shaped" as possible, avoiding narrow or sliver triangles.

\section{More Experimental Results}\label{more_results}
\subsection{Quantitative Results}
We present a detailed quantitative comparison of each scene with online methods including StreamRF, Dynamic3DGS and 3DGStream, in terms of rendering quality, storage efficiency and warping error, as shown in \cref{table:supple_comparison_table_online}. 
The results demonstrate that our method obtains the best rendering performance (entire image) and storage efficiency across all scenes and gives improved rendering quality (dynamic region) and temporal consistency in the majority of scenes.

% Our method shows the best performance in terms of rendering quality and storage efficiency, and the best or second warping error in all scenes. 

% \textcolor{red}{adding several texts to say comparing results.}

\begin{figure}[t]

  \centering
  \includegraphics[width=\linewidth]{figure_supple/motion_nums.png}
   \caption{Number of total 3DGs and motion-related 3DGs of each scene on the N3DV dataset.
   }
   \label{fig:quantity_3DGs}
\end{figure}

\subsection{Qualitative Results}
We provide a supplementary video demonstrating the dynamic novel view synthesis results, including the comparisons with other \textit{online} methods.

Additionally, We provide detailed visualisation results of the maintext ablation study (\cref{table:Ablation_architecture,table:Ablation_NOL}). We merge rows 2-3 in \cref{table:Ablation_NOL} with \cref{table:Ablation_architecture} to eliminate redundancy. As shown in the \cref{fig:visual_ablation}, our method achieves competitive visual effects (see flaming gun and dog's tongue), while within minimum storage and training parameters.

% We provide all dynamic novel view synthesis videos on supplementary files, including the results of all streamable methods.

\subsection{Metrics}\label{more_metrics}
The quantitative evaluation of rendering performance is presented using the PSNR metric, calculated for both the entire image and the dynamic regions, denoted as PSNR($\cdot$ / $\cdot$) in \cref{table:supple_comparison_table_online}. As illustrated in \cref{fig:dynamic_region}, the dynamic regions are defined through manually annotated bounding boxes.

% we report the rendering performance with the PSNR from the entire image and the dynamic regions of the image, as shown in \cref{table:supple_comparison_table_online} PSNR($\cdot$ / $\cdot$). The dynamic regions are manually labeled in box areas as shown in \cref{fig:dynamic_region}.

\subsection{Quantity of motion-related 3DGs}
\cref{fig:quantity_3DGs} illustrates the average number of the initial 3DGs and the motion-related 3DGs ($G_m$) across all 300 frames for each scene in the N3DV dataset. 
The results demonstrate that $G_m$ constitutes about $1/7-1/5$ of the total 3DGs, representing a significant reduction in training/storage requirements.
Notably, in scenes with a large number of initial 3DGs, such as \textit{coffee$\_$martini} and \textit{flame$\_$salmon$\_$1}, the number of $G_m$ drops to approximately $1/7$ of the total 3DGs, demonstrating enhanced storage efficiency and temporal consistency, as evidenced in \cref{table:supple_comparison_table_online}.

% It can be seen that the number of $G_m$ is much smaller than the total 3DGs number, which is about $1/6$~$1/3$. This verifies the training/storage efficiency of our method. In addition, for scenes with a large number of initial 3DGs, \eg \textit{coffee_martini} and \textit{flame_salmon_1}, the proportion of $G_m$ is smallest, about $1/6$, which indicates we have the improved storage efficiency and temporal consistency, as shown in\cref{table:supple_comparison_table_online}.}
% 图四给出初始的3DGs以及300帧中运动相关的3DGs的平均数量，从图四可以看出，运动相关的3DGs数量远小于总数，约为1/6~1/3。这验证了我们方法训练/存储的效率性。此外，对于初始高斯球数目越多的场景，如flame_samlon_1以及coffee_martini, 我们运动所需的高斯球占比总高斯球比例越低，可以获得好的存储效率以及时间连续性，如表所示。

% Exclude calculating the PNSR on the entire image, We additionally evaluate the PNSR in the dynamic regions, as shown in \cref{table:supple_comparison_table_online} PSNR($\cdot$ / $\cdot$). 
% We give the dynamic region of PSNR evaluation in \cref{fig:dynamic_region}, where the boxes are manually labeled dynamic regions.
% Specifically, we only evaluate the PNSR in the box, which is manually labeled dynamic region, as shown in \cref{fig:dynamic_region}.

\begin{figure}[t!]  % \begin{figure}[ht!]
	\centering
	\begin{subfigure}{\linewidth}
            \begin{minipage}[t]{0.327\linewidth}
                \centering
                \includegraphics[width=1\linewidth]{figure_supple/ab1/fig1.png}
                \caption{Tab.3 1st-row}
            \end{minipage}
            \begin{minipage}[t]{0.327\linewidth}
                \centering
                \includegraphics[width=1\linewidth]{figure_supple/ab1/fig2.png}
                \caption{Tab.3 2nd-row}
            \end{minipage}
            \begin{minipage}[t]{0.327\linewidth}
                \centering
                \includegraphics[width=1\linewidth]{figure_supple/ab1/fig3.png}
                \caption{Tab.3 3rd-row}
            \end{minipage}
        \end{subfigure}

        % \vspace{0.1cm}
	\begin{subfigure}{\linewidth}
            \begin{minipage}[t]{0.327\linewidth}
                \centering
                \includegraphics[width=1\linewidth]{figure_supple/ab1/fig4.png}
                 \caption{Tab.3 4th-row}
            \end{minipage}
            \begin{minipage}[t]{0.327\linewidth}
                \centering
                \includegraphics[width=1\linewidth]{figure_supple/ab1/fig5.png}
                \caption{Tab.3 5th-row}
            \end{minipage}
            \begin{minipage}[t]{0.327\linewidth}
                \centering
                \includegraphics[width=1\linewidth]{figure_supple/ab1/fig6.png}
                \caption{Tab.4 1st-row}
            \end{minipage}
        \end{subfigure}

        % \vspace{0.1cm}
	\begin{subfigure}{\linewidth}
            \begin{minipage}[t]{0.327\linewidth}
                \centering
                \includegraphics[width=1\linewidth]{figure_supple/ab1/fig7.png}
                 \caption{Tab.4 4th-row}
            \end{minipage}
            \begin{minipage}[t]{0.327\linewidth}
                \centering
                \includegraphics[width=1\linewidth]{figure_supple/ab1/fig8.png}
                \caption{Tab.4 5th-row}
            \end{minipage}
            \begin{minipage}[t]{0.327\linewidth}
                \centering
                \includegraphics[width=1\linewidth]{figure_supple/ab1/fig9.png}
                \caption{Ground Truth}
            \end{minipage}
        \end{subfigure}
       \caption{The visualization results of the maintext ablation study \cref{table:Ablation_architecture,table:Ablation_NOL}, where (e) is our method and (i) is Ground Truth. Others represent the ablation results.}
       \label{fig:visual_ablation}
\end{figure}

\begin{table}[!t]
% \vspace{-1.1em}
% \caption{The effectiveness of individual components. \colorbox{Magenta!30}{Pink} indicates the setting in this paper. Best performances are highlighted in bold.}
\caption{The effectiveness of individual components.  \textit{OFM}: Optical Flow Mask, \textit{TDM}: Temporal Difference Mask, \textit{CH}: Convex Hull, \textit{CA}: Clustering Algorithms, \textit{OP}: Optimization phase. \textit{Non-Motion-Mask}: Training process without motion masks (All 3DGs are treated as motion-related 3DGs).
\colorbox{Magenta!30}{Pink} indicates the setting in this paper. Best performances are highlighted in bold.}
\label{table:individual}

\centering 
\footnotesize
\begin{tabular}{c | c | c | c | c | c | c | c}
\Xhline{3\arrayrulewidth}
OFM & TDM & CH & CA & OP & PSNR$\uparrow$ & Storage$\downarrow$ & Ewarp$\downarrow$\\
\hline

\textcolor{red}{\ding{55}} & \textcolor{green}{\checkmark} & \textcolor{green}{\checkmark} & \textcolor{green}{\checkmark} & \textcolor{green}{\checkmark} & 33.98 & 1.24 & \textbf{0.0083} \\
\textcolor{green}{\checkmark} & \textcolor{red}{\ding{55}} & \textcolor{green}{\checkmark} & \textcolor{green}{\checkmark} & \textcolor{green}{\checkmark} & 33.80 & 1.64 & 0.0102 \\
\textcolor{green}{\checkmark} & \textcolor{green}{\checkmark} & \textcolor{red}{\ding{55}} & \textcolor{green}{\checkmark} & \textcolor{green}{\checkmark} & 33.85 & \textbf{1.03} & 0.0096 \\
\textcolor{green}{\checkmark} & \textcolor{green}{\checkmark} & \textcolor{green}{\checkmark} & \textcolor{red}{\ding{55}} & \textcolor{green}{\checkmark} & 34.29 & 3.22 & 0.0116 \\
\textcolor{green}{\checkmark} & \textcolor{green}{\checkmark} & \textcolor{green}{\checkmark} & \textcolor{green}{\checkmark} & \textcolor{red}{\ding{55}} & 33.51 & 1.36 & 0.0102 \\
    
\cellcolor{Magenta!30}\textcolor{green}{\checkmark} & \cellcolor{Magenta!30}\textcolor{green}{\checkmark} & \cellcolor{Magenta!30}\textcolor{green}{\checkmark} & \cellcolor{Magenta!30}\textcolor{green}{\checkmark} & \cellcolor{Magenta!30}\textcolor{green}{\checkmark} & \cellcolor{Magenta!30}\textbf{34.31} & \cellcolor{Magenta!30} 1.80 & \cellcolor{Magenta!30} 0.0104 \\

\hline
\multicolumn{5}{c|}{Non-Motion-Mask} & 34.24 & 5.17 & 0.0124 \\
    
\Xhline{3\arrayrulewidth}
\end{tabular}
\end{table}

\section{More Ablation Study}\label{more_ablation_study}
\textbf{Effect of individual components.}
To assess the individual impact of each proposed component, we carried out experiments with the removal of any single component. As illustrated in \cref{table:individual}, the removal of any single component results in degraded rendering performance. Most notably, the absence of clustering leads to substantially increased storage overhead and compromised temporal consistency.

\textbf{Effect of different thresholds for generating optical flow mask}. 
% To explore the impact of different thresholds $\tau$ on obtaining the optical flow mask, we conduct several experiments that set different $\tau$ for the optical flow maps. 
We conducted experiments with varying thresholds ($\tau$) to evaluate their effects on the generation of optical flow masks. As illustrated in \cref{fig:optical_thresholds}, we evaluated three threshold values: $\tau = 0.5$, $1.0$, and $1.5$. The experimental results show that a threshold of $\tau=1$ yields the most accurate motion detection results. Setting a lower threshold ($\tau = 0.5$) introduces false positives, misclassifying static objects like the curtain and the table as moving elements. Conversely, a higher threshold ($\tau=1.5$) results in incomplete motion detection, particularly evident in regions like human heads. 
Therefore, we adopted $\tau = 1.0$ in our implementation.
% Furthermore, even with a low threshold ($\tau=0.5$), tiny motions such as the moving flaming gun remained difficult to identify, highlighting the superiority of our approach that combines optical flow and temporal difference masks.
% As illustrated in the \cref{fig:optical_thresholds}, $\tau=1$ identifies the motion region more accurately. In contrast, a smaller threshold ($\tau=0.5$) mistakes static region for dynamic, such as the curtain and table, while a larger threshold ($\tau=1.5$) recognizes incomplete moving objects, such as the human head. In addition, it is difficult to distinguish the tiny motion even with a small threshold ($\tau=0.5$), such as the moving flaming gun, indicating the superiority of our motion mask which combined the optical flow mask and temporal difference mask.

\textbf{Effect of different thresholds for $\epsilon$}.
We conducted experiments with different thresholds ($\epsilon$ used in \cref{eq:DBSCAN}) to evaluate their effects on the experiment performance. As illustrated in \cref{table:epsilon}, the rendering quality rises as $\epsilon$ increases. When $\epsilon$ exceeds 2, there is a large decay in storage efficiency and temporal consistency. Thus we choose $\epsilon=2$ in our experiments.

% 我们执行实验在
\begin{figure}[t!]  % \begin{figure}[ht!]
	\centering
	\begin{subfigure}{\linewidth}
            \begin{minipage}[t]{0.31\linewidth}
                \centering
                \includegraphics[width=1\linewidth]{figure_supple/sup5_optical/fig1_t0.png}
                \caption{$I_{t-1}$}
            \end{minipage}
            \begin{minipage}[t]{0.31\linewidth}
                \centering
                \includegraphics[width=1\linewidth]{figure_supple/sup5_optical/fig2_t1.png}
                \caption{$I_{t}$}
            \end{minipage}
            \begin{minipage}[t]{0.31\linewidth}
                \centering
                \includegraphics[width=1\linewidth]{figure_supple/sup5_optical/fig3_final.png}
                \caption{Motion Mask}
            \end{minipage}
        \end{subfigure}

        \vspace{0.1cm}
	\begin{subfigure}{\linewidth}
            \begin{minipage}[t]{0.31\linewidth}
                \centering
                \includegraphics[width=1\linewidth]{figure_supple/sup5_optical/fig4_05.png}
                 \caption{$\tau=0.5$}
            \end{minipage}
            \begin{minipage}[t]{0.31\linewidth}
                \centering
                \includegraphics[width=1\linewidth]{figure_supple/sup5_optical/fig5_10.png}
                \caption{$\tau=1.0$}
            \end{minipage}
            \begin{minipage}[t]{0.31\linewidth}
                \centering
                \includegraphics[width=1\linewidth]{figure_supple/sup5_optical/fig6_15.png}
                \caption{$\tau=1.5$}
            \end{minipage}
        \end{subfigure}

       % \vspace{-0.5em}
       \caption{Illustration of the generation of optical flow mask. }
       \label{fig:optical_thresholds}
\end{figure}

\begin{table}[t!]
\caption{Ablation Study on $\epsilon$. \colorbox{Magenta!30}{Pink} indicates the setting in this paper. Best performances are highlighted in bold.} 
\label{table:epsilon}
\tabcolsep=0.45cm
\small
\centering 
\begin{tabular}{c | c | c | c }
\Xhline{3\arrayrulewidth}
Setting ($\epsilon$) & PSNR$\uparrow$ & Storage$\downarrow$ & Ewarp$\downarrow$\\
\hline

0.5 & 34.18 & \textbf{1.45} & \textbf{0.0097} \\
1.0 & 34.24 & 1.60 & 0.0100 \\

\cellcolor{Magenta!30} 2.0 & \cellcolor{Magenta!30} 34.31 & \cellcolor{Magenta!30} 1.80 & \cellcolor{Magenta!30} 0.0104 \\
5.0 & \textbf{34.36} & 3.05 & 0.0114 \\
10.0 & 34.32 & 3.22 & 0.0116 \\

\Xhline{3\arrayrulewidth}
\end{tabular}
\end{table}

\textbf{Effect of various numbers of 3DGs corresponding
to each pixel of GIM.}
To evaluate the impact of varying the number of 3DGs associated with each pixel in the GIM, we conducted experiments to determine it. 
The vanilla GIM utilizes the 3DG index with the highest weight during the alpha blending process. In contrast, our comparative analysis explored the effects of incorporating the top 2 to 5 weighted 3DGs, as shown in \cref{table:Ablation_GIM_number}, where \textit{GIM Top N} denotes the top N 3DGs based on weight ranking.
The results demonstrate that our method achieves superior training and storage efficiency as well as temporal consistency while maintaining comparable rendering quality.

% \textbf{The effectiveness of  with the method using total-variational (TV) loss.}
 \textbf{The effectiveness of the motion-related 3DGs.}
In order to improve the temporal consistency, the introduced MGStream utilizes the motion mask and the clustering-based convex hull algorithm to obtain the motion-related 3DGs, which are responsible for modeling the dynamic. 
In comparison, the regularization term, \textit{i.e.}, the grid-based total variation (TV) is employed to preserve the temporal consistency in the static regions \cite{4DGaussians,kplanes,fastdnerf}. 
To demonstrate the effectiveness of the motion-related 3DGs obtained, we employed the grid-based total variation (TV) to regularize the 3DGs instead of locating the motion-related 3DGs. 
The results in \cref{fig:tvloss} clearly show that the grid-based total variation (TV) struggles to  preserve the temporal consistency, and the introduced motion-related 3DGs contribute to modeling the dynamic.

\begin{figure}[t!]  % \begin{figure}[ht!]
	\centering
	\begin{subfigure}{\linewidth}
            \begin{minipage}[t]{0.31\linewidth}
                \centering
                \includegraphics[width=1\linewidth]{figure_supple/sup7_tvloss/GT.png}
                 \caption{GT}
            \end{minipage}
            \begin{minipage}[t]{0.31\linewidth}
                \centering
                \includegraphics[width=1\linewidth]{figure_supple/sup7_tvloss/ours.png}
                \caption{Ours}
            \end{minipage}
            \begin{minipage}[t]{0.31\linewidth}
                \centering
                \includegraphics[width=1\linewidth]{figure_supple/sup7_tvloss/tv.png}
                \caption{TV Loss Method}
            \end{minipage}
        \end{subfigure}

       % \vspace{-0.5em}
       \caption{Comparision with the method using TV loss. The \textcolor{blue}{blue} and \textcolor{red} {red} boxes show the quality of the novel synthesis, and \textcolor{green} {green} boxes represent the heatmap of the temporal variance in the static region, where the blacker the color, the smaller the variance.}
       \label{fig:tvloss}
\end{figure}

\begin{table}[!t]
\caption{Illustration of various numbers of 3DGs corresponding
to each pixel of GIM. \colorbox{Magenta!30}{Pink} indicates the setting in this paper. Best performances are highlighted in bold.} 
\label{table:Ablation_GIM_number}
\tabcolsep=0.3cm
\centering 
% \footnotesize
\small
\begin{tabular}{c | c | c | c | c}
\Xhline{3\arrayrulewidth}
GIM & PSNR$\uparrow$ & Storage$\downarrow$ & Train$\downarrow$ & \multirow{2}{*}{$E_{warp}\downarrow $}\\
(\textit{Top N}) & (db) & (MB) & (mins) & \\
    
\hline

\cellcolor{Magenta!30}{N=1} & \cellcolor{Magenta!30} 28.42 & \cellcolor{Magenta!30} \textbf{2.52} & \cellcolor{Magenta!30} \textbf{0.215} & \cellcolor{Magenta!30} \textbf{0.0088} \\
N=2 & 28.44 & 2.81 & 0.228 & 0.0094 \\
N=3 & 28.44 & 3.10 & 0.247 & 0.0097 \\
N=4 & 28.44 & 3.36 & 0.272 & 0.0101 \\
N=5 & \textbf{28.47} & 3.69 & 0.372 & 0.0103 \\

\Xhline{3\arrayrulewidth}
\end{tabular}
\end{table}
